# Supplementary material for: nBIIG: A Neural BI Insights Generation System for Table Reporting
Source: arXiv:2211.04417 source file (2022-11-08)
Supplement: Supplementary file 1 [file Appendix.tex]

\appendix
\label{Appendix}
\section{Appendix}

\subsection{Implementation Details}
\label{A: Implementation details}
\subsubsection{Training machinery}
All models were fine-tuned for 10 epochs and a batch size of $64$ (the maximum batch size that fits our largest model on our GPU). We used the \textit{adafactor} optimizer~\cite{shazeer2018adafactor}, with the default learning rate of $1\times10^{-4}$ and the common autoregressive cross entropy loss. Input and output sequence length were set to 64 tokens of the default models tokenizers.
A single NVIDIA A100 GPU was used for fine-tuning. All our pretrained models where taken from the \textit{huggingface-hub}\footnote{https://huggingface.co/models}. Our Implementation is based on Huggingface Transformers~\cite{wolf2019huggingface} version 4.20.1 and pytorch~\cite{paszke2019pytorch} version 1.9.0.

\begin{figure*}[t]
\begin{center}
  \includegraphics[width=1\textwidth]{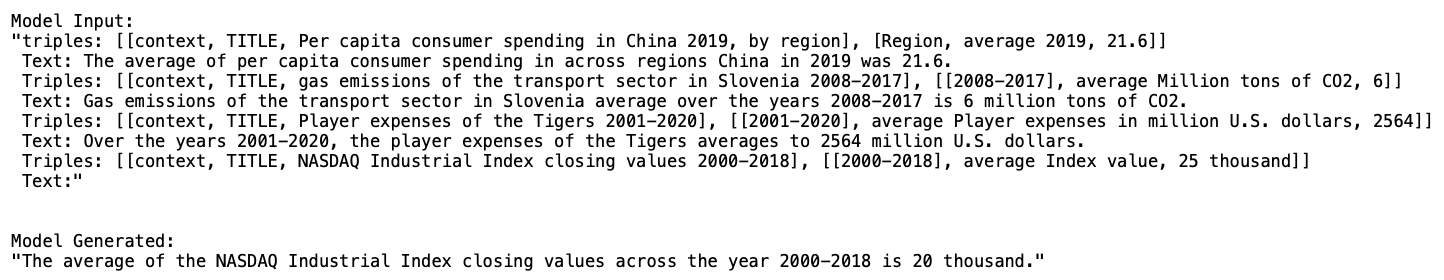}
 \end{center}
  \caption{Few-shot example for type AVERAGE.}~\label{fig:few-shot}
\end{figure*}

\begin{figure}
\begin{center}
  \includegraphics[width=1\columnwidth]{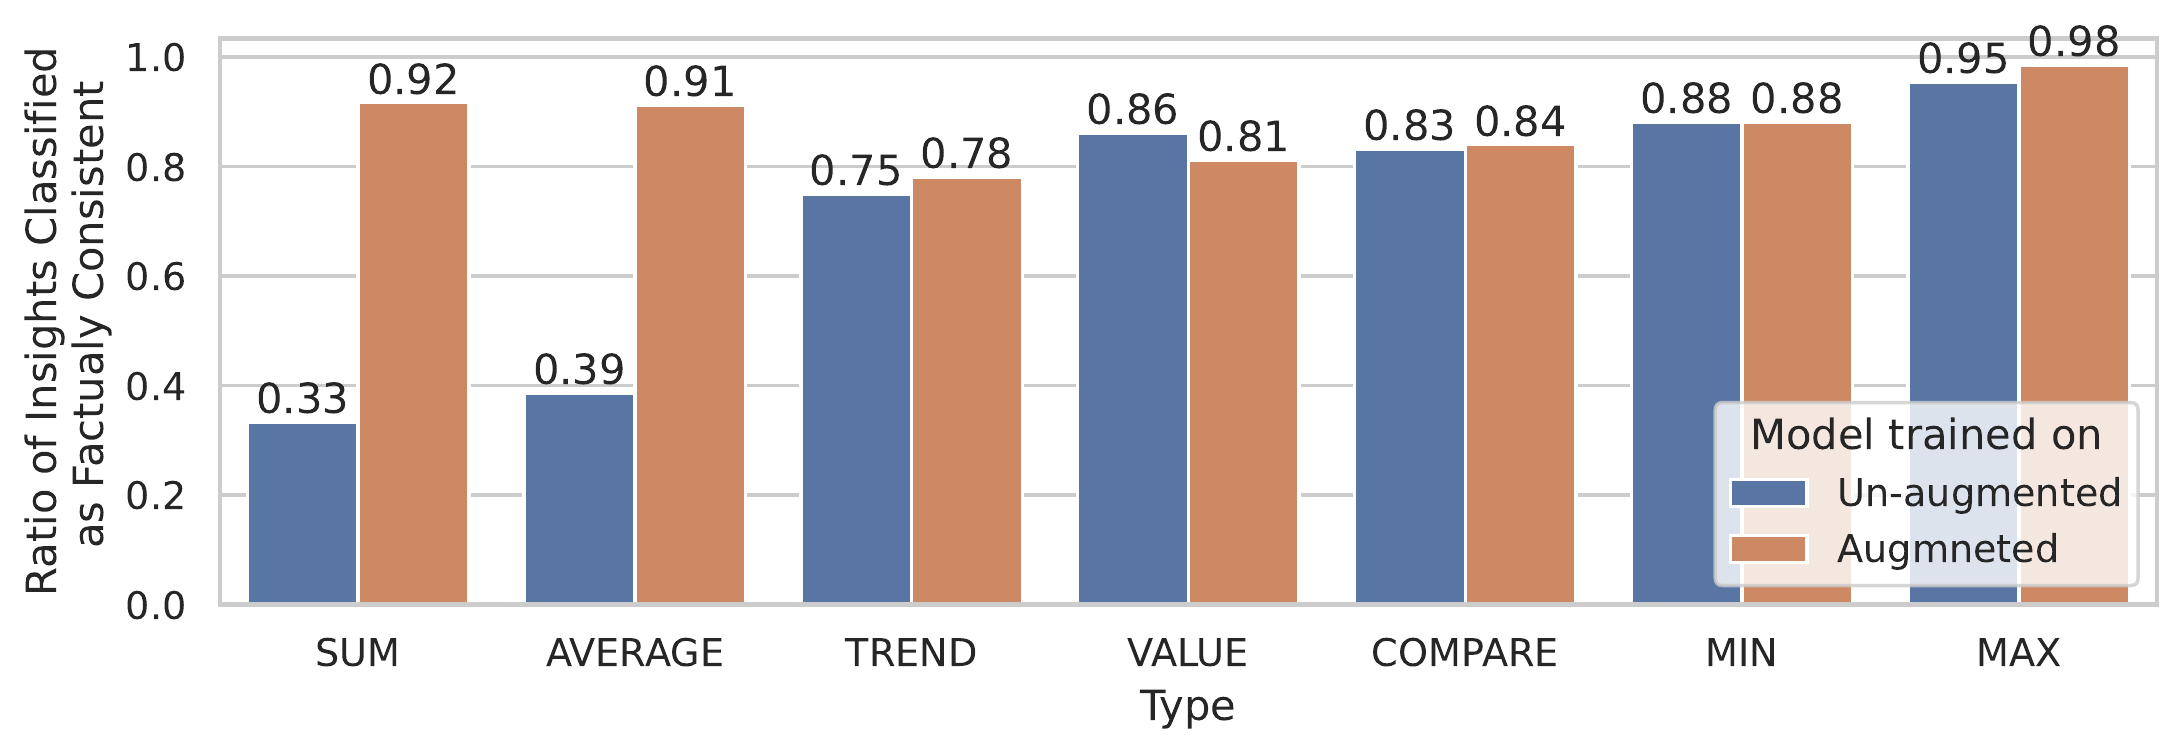}
 \end{center}
  \caption{\textbf{Ratio of insights classified as factually consistent, comparing model trained with augmented and un-augmented dataset:} SUM and AVERAGE show significant factuality improvement of $49\%$ and $42\%$, respectively.}
 \label{fig:aug_vs_unaug}
\end{figure}
